# Supplementary material for: DIMSpan - Transactional Frequent Subgraph Mining with Distributed In-Memory Dataflow Systems
Source: arXiv:1703.01910 source file (2017-03-06)
Supplement: Supplementary file 1 [file 80_appendix.tex]

\section*{Appendix - Disprove of Isomorphism-free Verification of MRFSE}
In the following, we provide a disprove by counterexample to show that the isomorphism-free verification of gSpan's minimum DFS codes \cite{yan2002gspan} proposed by \cite{lu2013efficiently} according to the information provided in the paper is not correct as it fails for subgraphs containing automorphisms. The author did not answer to a source code request. 

\subsection*{Definitions}
We first define graph, DFS code and embedding according to \cite{lu2013efficiently}:
\begin{small}

\begin{definition}
\textsc{(Graph)}. 
 A simple undirected vertex-labeled graph, in the following simply denoted by \textit{graph}, is a triple $G=\langle V, E, \lambda \rangle$ of vertice $V$, edges $E \subseteq \mathcal{P}(E) \mid \forall e \in E : |e| \in \{1,2\}$ and a labeling function $\lambda : (V \cup E) \rightarrow L$ associating a label $l \in L$ to every vertex and edge.
\end{definition}

\begin{definition}
\label{def:dfscode}\textsc{(DFS Code)}.
A \textit{DFS code} representing a pattern of $j$ vertices and $k$ edges ($j,k \geq 1$) is defined to be an $k$-tuple $C = \langle x_1,x_2,..,x_k \rangle$ of extensions, where each \textit{extension} is a pentuple $x =\langle t_a, t_b, l_a, l_e, l_b \rangle$ representing the traversal of an edge $e$ with label $l_e \in L$ from a \textit{start} vertex $v_a$ with label $l_a \in L$ to an \textit{end} vertex $v_b$ with $l_b \in L$ and their initial discovery times $t_a, t_b \in T \mid T = \langle 0, .., j \rangle$ where the vertex at $t=0$ is always the start vertex of the first extension. A DFS code $C_p$ will be considered to be the parent of a DFS code $C_c$, iff $\forall i \in \langle 1,..,k-1 \rangle : C_c.x_i = C_p.x_i$.
\end{definition} 

A \textit{minimum DFS code} is defined according to Definition \ref{def:mindfs}.

\begin{definition}
\textsc{(Embedding)}. 
Given a graph $G$ and a DFS code $C$, than an \textit{embedding} is defined to be an n-tuple $m = \langle v_t \mid t \in T \rangle$ of vertices and their index correponds to the initial discovery time. 
\end{definition}

% \textit{Lemma:}
% The recalculation of a graph's canonical label requires enumerating all subgraph automorphisms and thus contains the problem of isomorphism testing.
\end{small}

\subsection*{Proposition}
Due to the condition in line 10 of Algorithm 2 and Lemma V of  \cite{lu2013efficiently}, a pair of DFS code and embedding $g^{s}_{e}$ will only be added to the output, if there not already exists a pair in hashset $genG$ covering exactly the same edge set. In consequence, only the first $g^s_e$ for each distinct edge set will be added to the output. Thus, the authors propose that for every graph $G$ and every minimal $k$-edge DFS code $C_{min}$ it is possible to generate the complete set of minimal $k+1$-edge children based on exactly one embedding which maps a subgraph of $G$ to $C_{min}$.

\subsection*{Counterexample}
Given the two graphs $G_1,G_2$ of Figure \ref{fig:disprove}, in the 3rd iteration the two black-lined subgraphs are both represented by a single minimum DFS code $C^3_{min}$. After extending both by the red edges to the resulting minimal DFS code is $C^4_{min}$. Both minimum DFS codes are listed on top of Table \ref{tab:disprove}. The table further lists all 6 possible embeddings $m_{11},..,m_{16}$ and $m_{21},..,m_{16}$ for each of the two graphs before and after pattern growth. We see not all possible extensions lead to a minimum DFS code (e.g., $m_{11}$ does not). These are the ones that have to be filtered out in a verification step to be neither added to the result nor to become extended in the subsequent iteration.

In \cite{lu2013efficiently}, only the first discovered embedding for each distinct edge subset and minimum DFS code is stored, i.e., only one of $m_{11},..,m_{16}$ and one of $m_{21},..,m_{16}$. Let $m_{11}$ and $m_{21}$ be the stored ones, than the frequency of $C^4_{min}$ will be incorrect as the false positive code of $m_{11}$ will be counted instead. Let $m_{11}$ and $m_{22}$ be the stored ones than the correct minimum DFS code will never be generated. We see, a single embedding per distinct edge set and DFS code cannot guarantee to generate all minimal children. Our counterexample shows that extending DFS codes using an isomorphism-free append-only approach based on only a single embedding cannot guarantee for the correct result. 

\subsection*{Contradiction}
The isomorphism-free verification of \cite{lu2013efficiently} potentially fails for all subgraphs containing at least one automorphism. Subgraphs similar to our counterexample occur inter alia in molecular databases, for example, cycloalkanes\footnote{\url{https://en.wikipedia.org/wiki/Cycloalkane}}.

\begin{figure}[t]
  \vspace{-3mm}
  \caption{Illustration of our couterexample showing two graphs $G_1,G_2$ with each one $3$-edge subgraph containing automorphisms (black lines) and an extension to a $4$-edge subgraph (red lines). Roman numbers are vertex identifiers.}
	\label{fig:disprove}
	\centering
  \includegraphics[width=0.45\textwidth]{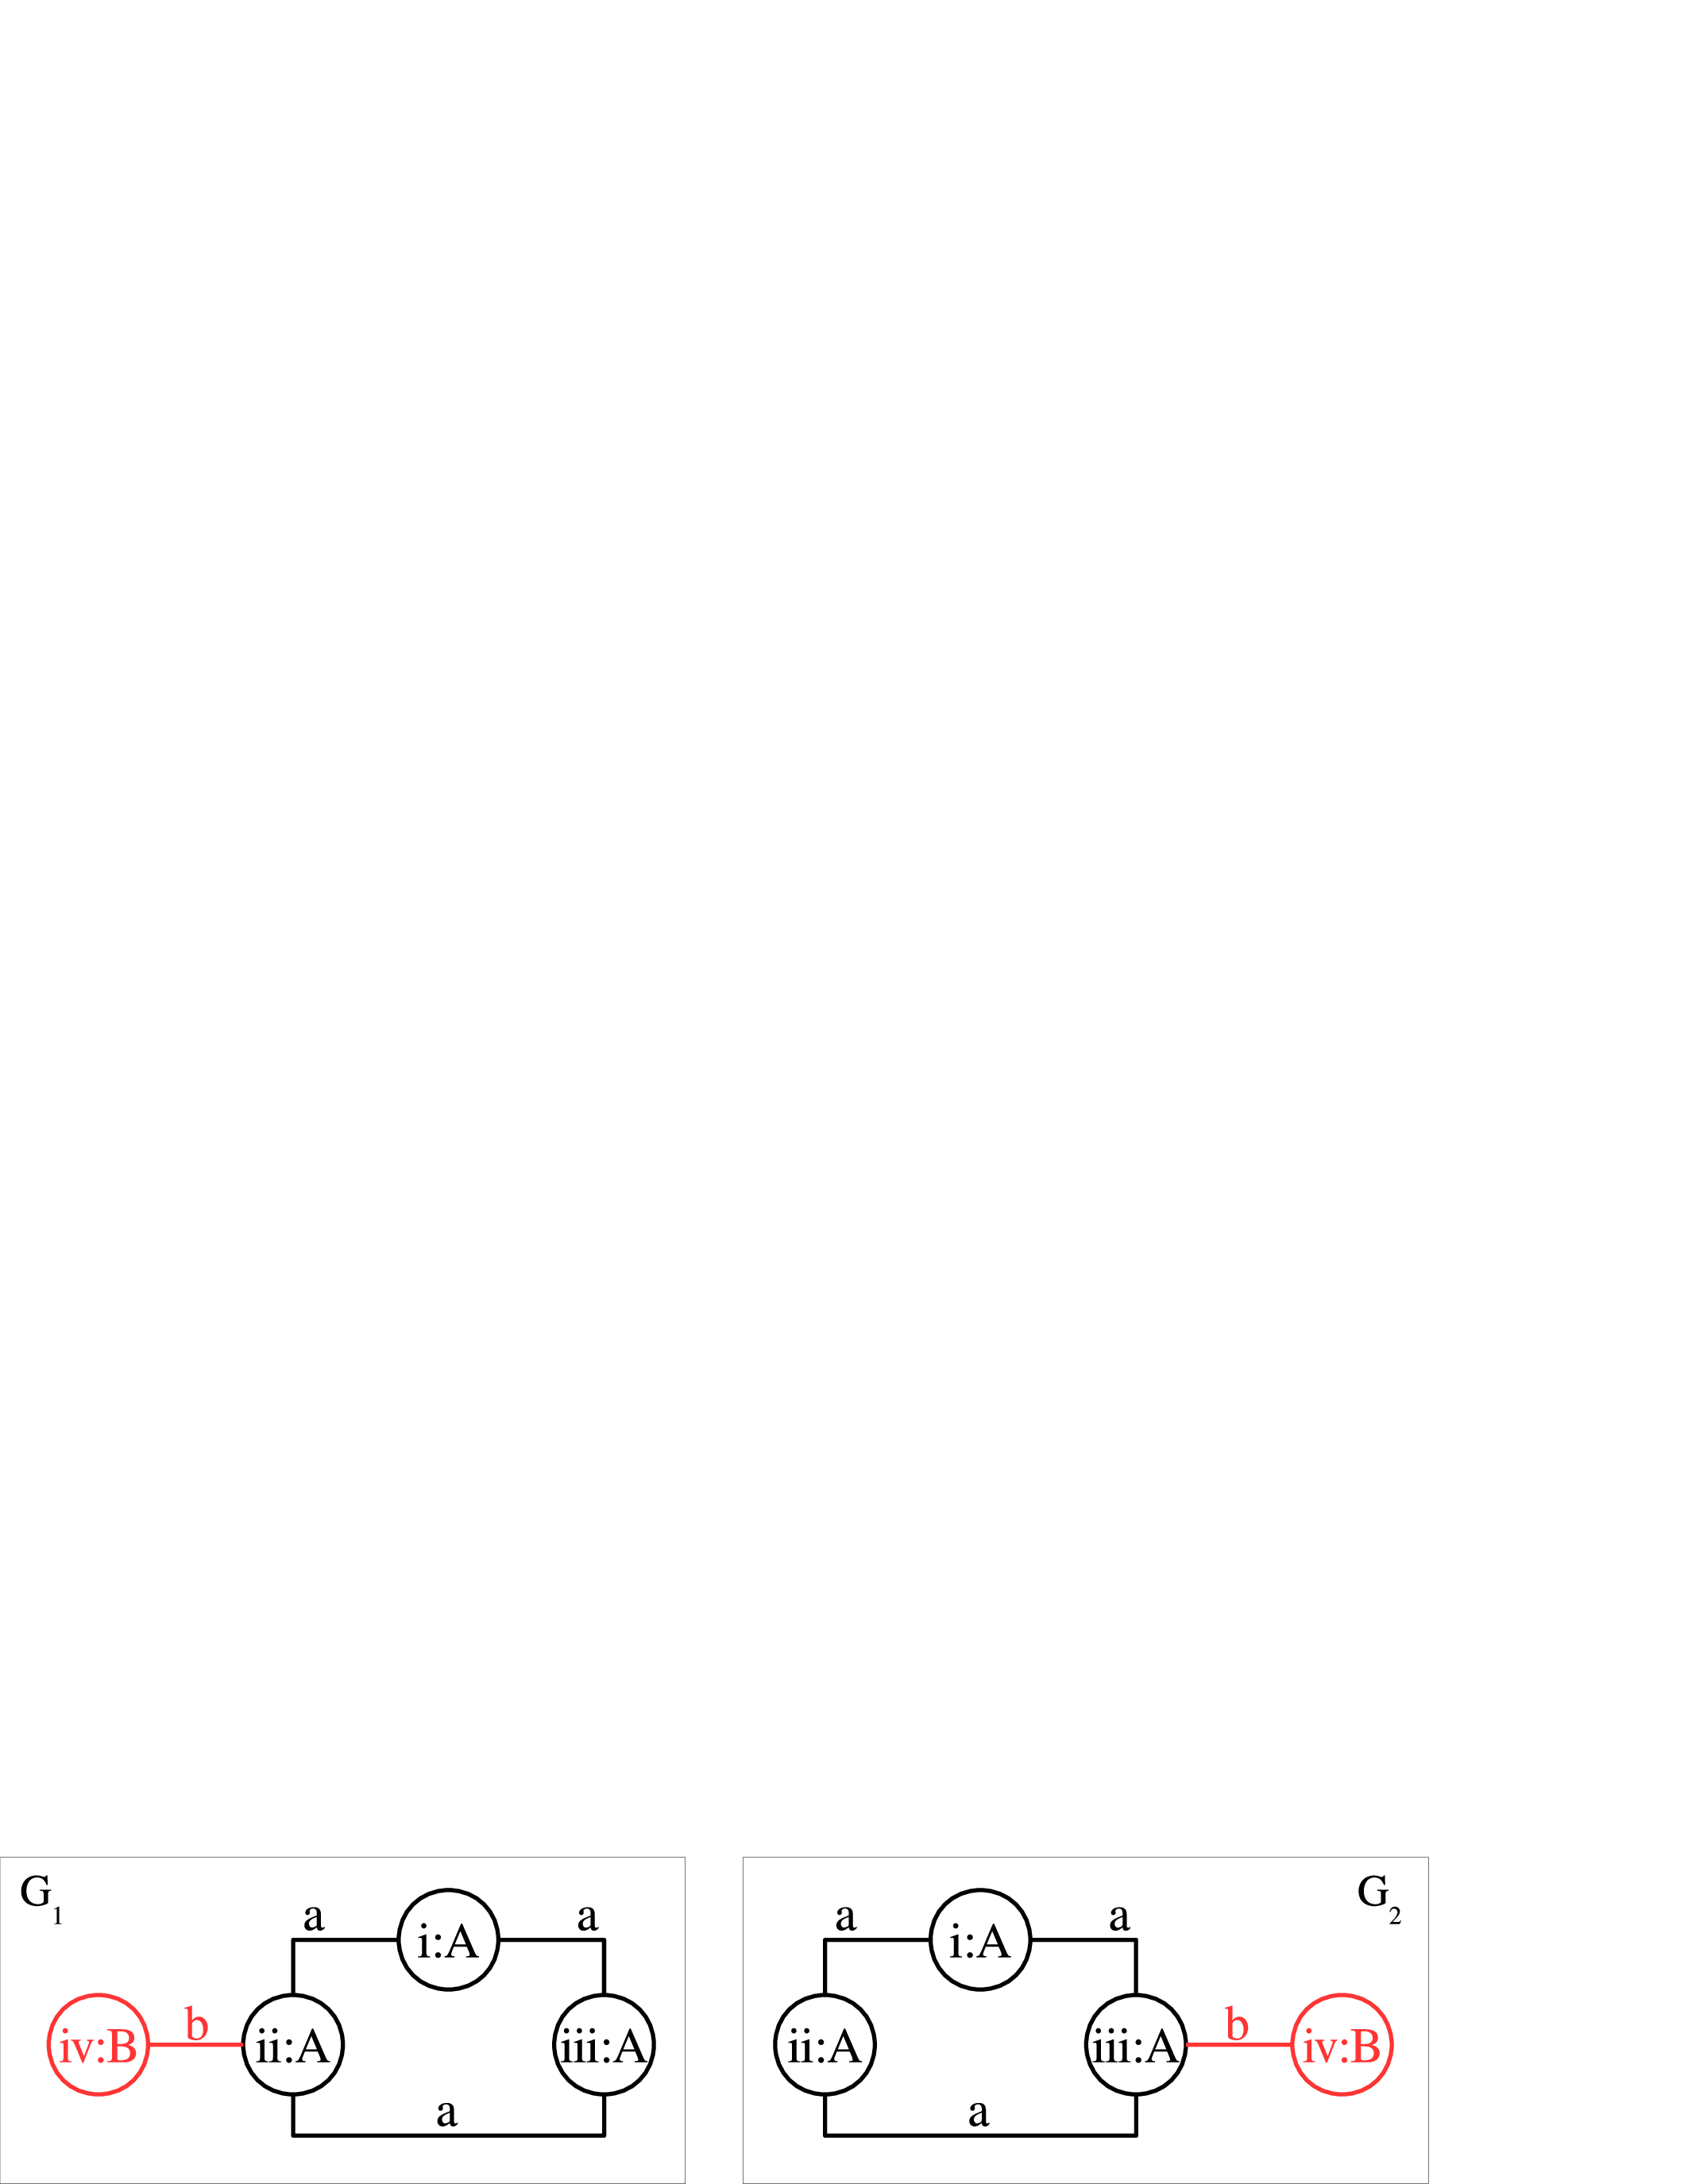}
\end{figure}

\begin{table}[t]
\caption{Embeddings and DFS codes during the pattern growth from $3$-edge subgraphs (black lines) to $4$-edge subgraphs (red lines) in the graphs of Figure \ref{fig:disprove}.}
\label{tab:disprove}
\begin{center}

\begin{tabular}{lllll}
 $C^3_{min}$ & \multicolumn{4}{l}{ $\langle \langle 0,1,A,a,A \rangle, \langle 1,2,A,a,A \rangle, \langle 2,0,A,a,A \rangle \rangle$} \\
  $C^4_{min}$ & \multicolumn{4}{l}{ $\langle \langle 0,1,A,a,A \rangle, \langle 1,2,A,a,A \rangle, \langle 2,0,A,a,A \rangle, \langle 2,3,A,b,B \rangle \rangle$} \\
  \\
 \hline
 & $k$-edge emb. & $k+1$-edge emb. & extension & minimal \\
\hline
$G_1$ : \\
$m_{11}$ & $\langle i,ii,iii \rangle$ & $\langle i,ii,iii, iv \rangle$ & $\langle 1,3,A,b,B \rangle$ & no\\
$m_{12}$ & $\langle i,iii,ii \rangle$ & $\langle i,iii,ii, iv \rangle$ & $\langle 2,3,A,b,B \rangle$ & yes\\
$m_{13}$ & $\langle ii,i,iii \rangle$ & $\langle ii,i,iii, iv \rangle$ & $\langle 0,3,A,b,B \rangle$ & no\\
$m_{14}$ & $\langle ii,iii,i \rangle$ & $\langle ii,iii,i, iv \rangle$ & $\langle 0,3,A,b,B \rangle$ & no\\
$m_{15}$ & $\langle iii,i,ii \rangle$ & $\langle iii,i,ii, iv \rangle$ & $\langle 2,3,A,b,B \rangle$ & yes\\
$m_{16}$ & $\langle iii,ii,i \rangle$ & $\langle iii,ii,i, iv \rangle$ & $\langle 1,3,A,b,B \rangle$ & no\\

\hline
$G_2$ : \\
$m_{21}$ & $\langle i,ii,iii \rangle$ & $\langle i,ii,iii, iv \rangle$ & $\langle 2,3,A,b,B \rangle$ & yes\\
$m_{22}$ & $\langle i,iii,ii \rangle$ & $\langle i,iii,ii, iv \rangle$ & $\langle 1,3,A,b,B \rangle$ & no\\
$m_{23}$ & $\langle ii,i,iii \rangle$ & $\langle ii,i,iii, iv \rangle$ & $\langle 2,3,A,b,B \rangle$ & yes\\
$m_{24}$ & $\langle ii,iii,i \rangle$ & $\langle ii,iii,i, iv \rangle$ & $\langle 1,3,A,b,B \rangle$ & no\\
$m_{25}$ & $\langle iii,i,ii \rangle$ & $\langle iii,i,ii, iv \rangle$ & $\langle 0,3,A,b,B \rangle$ & no\\
$m_{26}$ & $\langle iii,ii,i \rangle$ & $\langle iii,ii,i, iv \rangle$ & $\langle 0,3,A,b,B \rangle$ & no\\
 \hline
\end{tabular}

\end{center}
\end{table}
